# Supplementary material for: Swap Regret and Correlated Equilibria Beyond Normal-Form Games
Source: arXiv:2502.20229 source file (2025-02-27)
Supplement: Supplementary file 1 [file appendix-related.tex]

\section{Additional Related Work}\label{app:related-work}
